# Supplementary material for: Attack-in-the-Chain: Bootstrapping Large Language Models for Attacks Against Black-box Neural Ranking Models
Source: arXiv:2412.18770 source file (2024-12-25)
Supplement: Supplementary file 1 [file appendix.tex]

% \iffalse
\clearpage
\appendix
\section{Appendix}

\subsection{Complete attack evaluation results}
The attack performance of AttChain and baselines on Mixture target documents is shown in Table \ref{mix}.

\begin{table*}[!htb]
\centering
   \setlength\tabcolsep{20pt}
  	\begin{tabular}{l  c c c  c c c}
  \toprule
  Method & \multicolumn{3}{c}{MS MARCO} & \multicolumn{3}{c}{TREC2019}  \\ 
  \cmidrule(r){1-4} \cmidrule(r){5-7} 
   \textbf{BERT}  & ASR & Boost & T10R & ASR & Boost & T10R \\ 
       \midrule
TS & 94.3 & 53.6 & 54.0 & 95.1 & 51.0 & 51.8 \\
PRADA  & 88.2 & 41.1 & 39.0 & 87.1 & 39.5 & 37.2  \\
PAT   & 90.9 & 48.1 & 48.0 & 89.2 & 44.6 & 45.5 \\
IDEM   & 95.1 & 54.9 & 55.6 & 93.4 & 51.4 & 52.0 \\
\midrule
AttChain$_\mathrm{Llama}$  & 99.6 & 64.6\rlap{$^{\ast}$} & 63.0\rlap{$^{\ast}$} & 98.8\rlap{$^{\ast}$} & 62.4\rlap{$^{\ast}$} & 59.9\rlap{$^{\ast}$} \\
AttChain$_\mathrm{GPT}$  & \textbf{99.8} & \textbf{67.7}\rlap{$^{\ast}$} & \textbf{66.7}\rlap{$^{\ast}$} & \textbf{99.5}\rlap{$^{\ast}$} & \textbf{65.9}\rlap{$^{\ast}$} & \textbf{63.5}\rlap{$^{\ast}$} \\
AttChain$_\mathrm{-CoT}$  & 97.5 & 52.1 & 54.3 & 97.2 & 48.3 & 50.5 \\
AttChain$_\mathrm{-dynamic}$  & 99.4 & 63.0\rlap{$^{\ast}$} & 63.3\rlap{$^{\ast}$} & 99.4\rlap{$^{\ast}$} & 62.2\rlap{$^{\ast}$} & 60.5\rlap{$^{\ast}$} \\
\midrule
   \textbf{PROP}  & ASR & Boost & T10R & ASR & Boost & T10R \\ 
       \midrule
TS & 94.4 & 52.8 & 52.4 & 95.3 & 50.2 & 50.1 \\
PRADA  & 85.6 & 38.9 & 37.2 & 83.0 & 37.0 & 34.3 \\
PAT   & 89.9 & 46.1 & 46.2 & 86.6 & 41.2 & 42.8 \\
IDEM   & 94.1 & 51.9 & 53.2 & 92.9 & 50.6 & 50.1 \\
\midrule
AttChain$_\mathrm{Llama}$  & 99.0 & 63.1\rlap{$^{\ast}$} & 61.6\rlap{$^{\ast}$} & 98.4\rlap{$^{\ast}$} & 61.9\rlap{$^{\ast}$} & 59.1\rlap{$^{\ast}$} \\
AttChain$_\mathrm{GPT}$ & \textbf{99.8} & \textbf{66.2}\rlap{$^{\ast}$} & \textbf{65.0}\rlap{$^{\ast}$} & \textbf{98.8}\rlap{$^{\ast}$} & \textbf{65.0}\rlap{$^{\ast}$} & \textbf{61.8}\rlap{$^{\ast}$} \\
AttChain$_\mathrm{-CoT}$  & 96.5 & 50.1 & 51.3 & 96.6 & 47.8 & 48.5 \\
AttChain$_\mathrm{-dynamic}$  & 99.7 & 61.0\rlap{$^{\ast}$} & 60.6\rlap{$^{\ast}$} & 98.5\rlap{$^{\ast}$} & 62.2\rlap{$^{\ast}$} & 58.9\rlap{$^{\ast}$} \\
\midrule
   \textbf{RankLLM} & ASR & Boost & T10R & ASR & Boost & T10R \\ 
       \midrule
TS & 94.6 & 48.7 & 49.6 & 92.6 & 44.1 & 44.6 \\
PRADA  & 80.5 & 35.8 & 33.5 & 80.9 & 33.5 & 33.3 \\
PAT   & 85.4 & 41.8 & 43.7 & 84.9 & 38.9 & 38.8 \\
IDEM   & 92.3 & 49.0 & 50.2 & 89.2 & 48.0 & 48.6 \\
\midrule
AttChain$_\mathrm{Llama}$  & 96.3 & 59.6\rlap{$^{\ast}$} & 55.7\rlap{$^{\ast}$} & 96.7\rlap{$^{\ast}$} & 59.1\rlap{$^{\ast}$} & 57.7\rlap{$^{\ast}$} \\
AttChain$_\mathrm{GPT}$  & \textbf{97.5} & \textbf{62.0}\rlap{$^{\ast}$} & \textbf{59.5}\rlap{$^{\ast}$} & \textbf{97.2}\rlap{$^{\ast}$} & \textbf{61.1}\rlap{$^{\ast}$} & \textbf{59.4}\rlap{$^{\ast}$} \\
AttChain$_\mathrm{-CoT}$  & 91.2 & 51.8 & 49.3 & 92.8 & 48.0 & 49.7 \\
AttChain$_\mathrm{-dynamic}$  & 96.6 & 59.6\rlap{$^{\ast}$} & 57.1\rlap{$^{\ast}$} & 96.5\rlap{$^{\ast}$} & 58.4\rlap{$^{\ast}$} & 57.0\rlap{$^{\ast}$} \\
\bottomrule
    \end{tabular}
\caption{Attack performance of AttChain and baselines on Mixture target documents; $\ast$ indicates significant improvements over the best baseline ($p \le 0.05$).}
\label{mix}
\end{table*}
